# Supplementary material for: Large-Scale Contextual Market Equilibrium Computation through Deep Learning
Source: arXiv:2406.15459 source file (2025-04-21)
Supplement: Supplementary file 1 [file Pseudocodes.tex]

\section{Training procedure for MarketFCNet}
\label{app:pseudocodes}
\subsection{Pseudocodes for MarketFCNet}

\begin{algorithm}[H]
\nextfloat
\caption{MarketFCNet}
\begin{algorithmic}
\STATE \textbf{Input:} An oracle of buyer sampler $b \sim F(b)$, goods $g_1,...,g_m$, batch size $M,N$, second-order parameter $\rho$, iteration $K$, step size for $(\beta_t)_{t=1}^\infty$.
\STATE \textbf{Output:} Allocation network $x(b,g;\theta)$, price $p_j$ for each good $g_j$
\STATE Initialize an allocation network $x(b,g;\theta)$ and multipliers $\{\lambda_j\}_\jinm$.
\FOR{$t = 1,2,...$ until converged}
    \FOR{$k = 1,2,... K$}
        \STATE Get an unbiased estimator $SG \approx \nabla_\theta \calL_\rho(\theta;\bmlam)$ with batch size $M$.
        \STATE Optimize $\theta$ with $Optimizer(\theta, SG)$.
    \ENDFOR
    \FOR{$j=1,...,m$}
        \STATE Get an unbiased estimator $\Delta \lambda_j \approx \rho (\bbE_{b}[x(b,g_j;\theta)] - 1 )$ with batch size $N$.
        \STATE Updates $\lambda_j$ with $\lambda_j \leftarrow \lambda_j + \beta_t \Delta \lambda_j $.
    \ENDFOR
\ENDFOR
\STATE \textbf{return:} $x(b,g;\theta)$: allocation network, $\{\lambda_j\}_\jinm$: price for good $g_j$.
\end{algorithmic}
\end{algorithm}

% \subsection{Pseudocodes for MarketTransNet}

% \begin{algorithm}[H]
% \caption{MarketTransNet}
% \begin{algorithmic}
% \STATE \textbf{Input:} number of buyers $n$, number of goods $m$, batch size $M$.
% \STATE \textbf{Output:}Transformer network $\calX(\bmb,\bmg;\theta)$ including allocation $\bmx(\bmb,\bmg;\theta)$ and price $\bmP(\bmb,\bmg;\theta)$
% \STATE Initialize a transformer network $\calX(\bmb,\bmg;\theta)$.
% \FOR{$t = 1,2,...$ until converged}
%     \STATE Generate $M$ batch of random market instance with $n$ buyers and $m$ goods.
%     \STATE Compute the loss function $\text{Nash-Gap}(\theta)$ on these instances.
%     \STATE Compute the gradient $Gradient = \nabla_\theta \text{Nash-Gap}(\theta)$.
%     \STATE Update $\theta$ with $Optimizer(\theta, Gradient)$.
% \ENDFOR
% \STATE \textbf{return:}$\calX(\bmb,\bmg;\theta)$: Transformer network that can determine allocation and price for one market.
% \end{algorithmic}
% \end{algorithm}
