# Supplementary material for: Large-Scale Contextual Market Equilibrium Computation through Deep Learning
Source: arXiv:2406.15459 source file (2025-04-21)
Supplement: Supplementary file 2 [file Transformer_Architecture.tex]

\section{Transformer Architecture}
\label{app:trans-architecture}

\subsection{Transformer Architecture}
\begin{figure}[t]
    \centering
    \caption{The architecture of MarketTransNet}
    \includegraphics[width=1\textwidth]{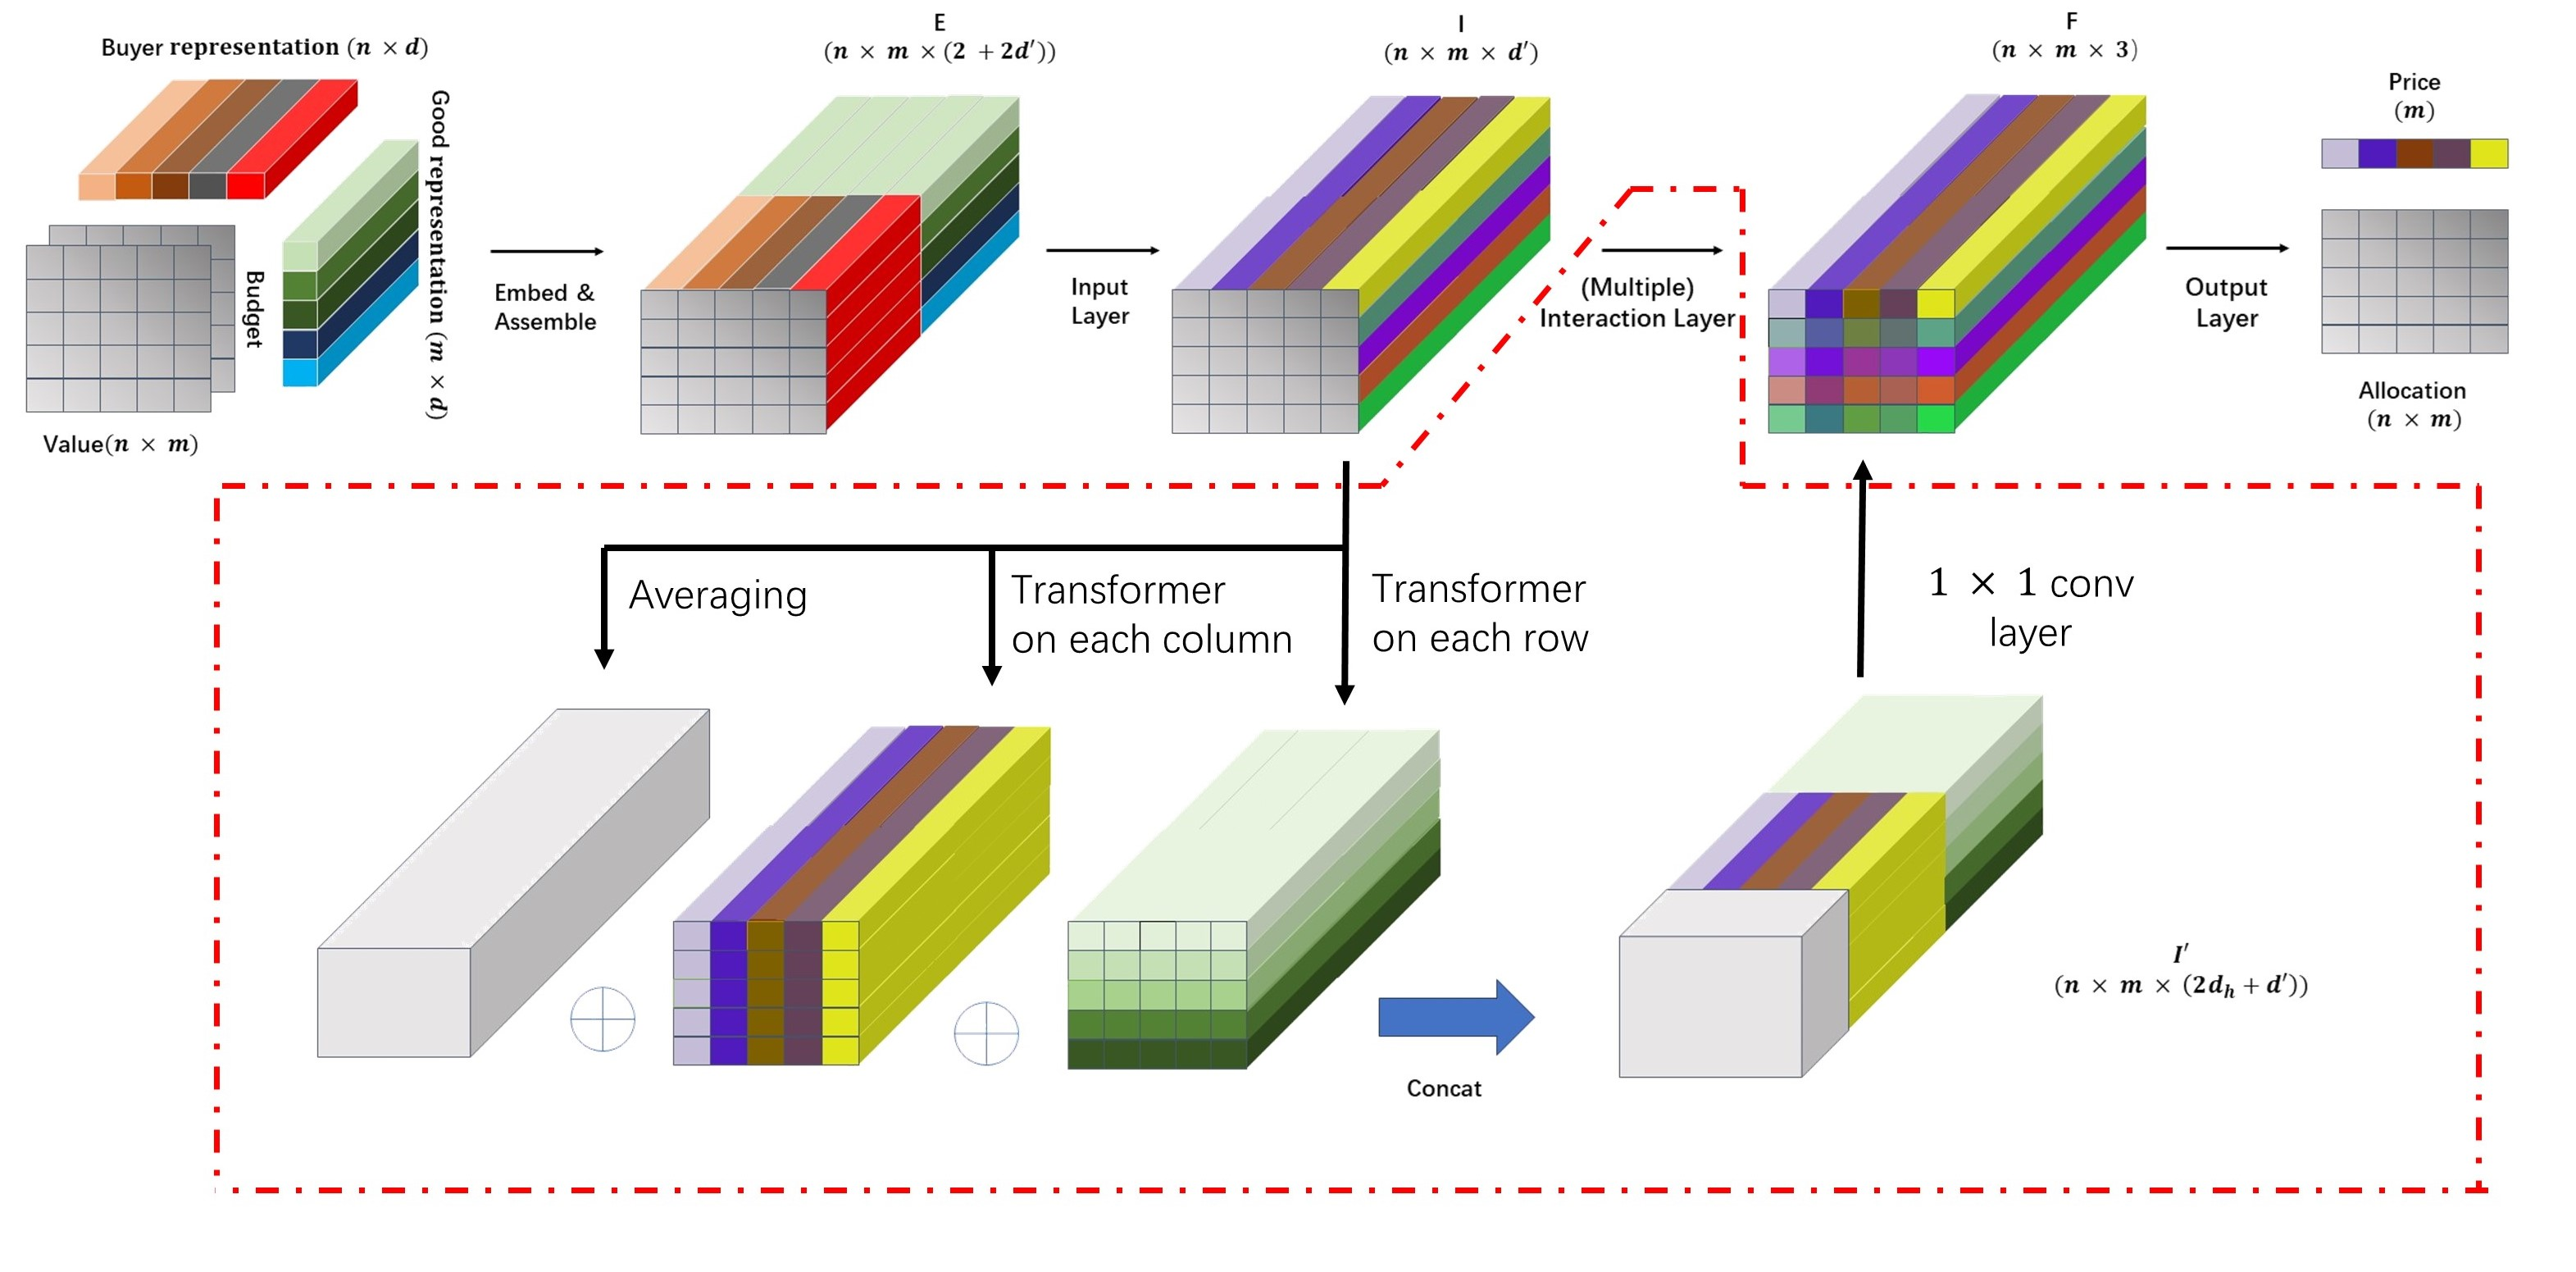}
    \label{fig:enter-label}
\end{figure}

\cref{fig:enter-label} illustrates the architecture of MarketTransNet, which is designed to model the market equilibrium by processing a comprehensive set of inputs: the value profile $\bmv \in \bbR^{n\times m}$, the budget vector $\bm{B} \in \calR^{n}$ for buyers, buyer-representations $\bmb \in \bbR^{n \times d}$, and good-representations $\bmg \in \calR^{m \times d}$. Initially, the input layer synthesizes the information pertaining to buyers and goods to constitute buyer-item pairs, each characterized by a feature dimension $\bmd$, resulting in a tensor $I \in \calR^{n\times m \times d}$.

Subsequently, these synthesized pairs undergo a series of mutual computations within multiple attention layers, fostering an intricate understanding of the interactions between buyers and goods. The endpoint of this process is represented by the final interaction layer, which yields a global feature map $F \in \calR^{n\times m \times 2}$. 

This feature map encapsulates the critical information required to deduce the final allocation result $\bmg(\bmp,\bmq;\theta)$ and the corresponding price vector $\bmp(\bmb,\bmg;\theta)$. These outputs are derived while adhering to the market constraints, specifically ensuring that the sum of allocations for each good equals the number of buyers ($\sum{\bmx_{ij}=n}$) and that each allocation $\bmx_{ij}$ remains positive ($\bmx_{ij}>0$). This structured approach enables MarketTransNet to effectively model and solve for market equilibria, leveraging the complex interdependencies encoded within the feature representations of buyers and goods.

\subsection{Input Layer}

For ease of calculation, we broadcast buyers' budget $\bm{B}_{i}$ to every good j with same value to get compatible shapes. By concatenating the budget of buyer i $\bm{B}_{ij}$, the valuation of buyer i over the good j $\bmv_{ij}$ and representation $\bmb_{i},\bmg_{j}$ into a vector, we construct the initial representation for each buyer-good pair E: 
% $$E_{i,j}= [\bm{B}_{ij};\bmv_{ij};\bmb_{ij};\bmg_{ij}] \in \bbR^{1+1+d_{\bmb}+d_{\bmg}}$$
\begin{align}
    E_{i,j}= [\bm{B}_{ij};\bmv_{ij};\bmb_{ij};\bmg_{ij}] \in \bbR^{1+1+d_{\bmb}+d_{\bmg}}
\end{align}
afterwards, two 1 × 1 convolutions with a ReLU activation are applied to E and reduce the representation dimension of E from $ 2 + d_{\bmb} + d_{\bmg}$ to $d-2$. after that, we concatenating new d-2 dimensional vector $E^{\prime}$ with the budget $\bm{B}$ and valuation $\bmv$.
% $$ I = [\bm{E^{\prime}};\bm{B};\bmv] \in \bbR^{n \times m \times d}$$
\begin{align}
    I = [\bm{E^{\prime}};\bm{B};\bmv] \in \bbR^{n \times m \times d}
\end{align}
In this way the input vectors of the network are unified to a buyer-good pair with representation dimension $\bbR^{d}$. 

\subsection{Interaction Layer}

The interaction layer is built based upon transformer model \citep{duan2022context}, which can be used to capture the high-order feature interactions of input through the multi-head self-attention module.

Initially, for each buyer $i$, the model captures the dynamics of its interactions with the complete set of $m$ goods. This is achieved through a transformer applied to the $i$-th row of matrix $I$ (expressed as $I_{i,\cdot} \in \bbR^{m \times d_h}$):

% $$
% I^{\text{row}}_{i,\cdot} = \text{transformer}(I_{i,\cdot}) \in \bbR^{m \times d_h}, \quad \forall i \in N,
% $$
\begin{align}
    I^{\text{row}}_{i,\cdot} = \text{transformer}(I_{i,\cdot}) \in \bbR^{m \times d_h}, \quad \forall i \in N,
\end{align}

Here, $d_h$ symbolizes the dimensionality of the hidden nodes within the MLP segment of the transformer. 

In a symmetrical fashion, for every good $j$, the model delineates its interactions with the entirety of $n$ buyers (represented as $I_{\cdot,j} \in \bbR^{n \times d_h}$):

% $$
% I^{\text{column}}_{\cdot,j} = \text{transformer}(I_{\cdot,j}) \in \bbR^{n \times d_h}, \quad \forall j \in M.
% $$
\begin{align}
    I^{\text{column}}_{\cdot,j} = \text{transformer}(I_{\cdot,j}) \in \bbR^{n \times d_h}, \quad \forall j \in M.
\end{align}

Following these interaction processes, the aggregate information pertaining to each pair of buyer and good is derived by averaging the feature set:

% $$
% e^{\text{global}} = \frac{1}{nm} \sum_{i=1}^{n} \sum_{j=1}^{m} I_{ij} \in \bbR^{d}.
% $$
\begin{align}
    e^{\text{global}} = \frac{1}{nm} \sum_{i=1}^{n} \sum_{j=1}^{m} I_{ij} \in \bbR^{d}.
\end{align}
Combining $I^{\text{row}}$, $I^{\text{column}}$, and $e^{\text{global}}$ together, we derive new features $I^{\prime}_{ij}$ for each buyer-good pair:
% $$
% I^{\prime}_{ij} := [I^{\text{row}}_{ij} ; I^{\text{column}}_{ij} ; e^{\text{global}}] \in \mathbb{R}^{2d_h + d}.
% $$
\begin{align}
    I^{\prime}_{ij} := [I^{\text{row}}_{ij} ; I^{\text{column}}_{ij} ; e^{\text{global}}] \in \mathbb{R}^{2d_h + d}.
\end{align}

Conclusively, Using the same technique above in input layer for compressing feature dimensions, we convert the output dimension to $d_{out}=2$:
% $$
% F = \text{Conv}(\text{ReLU}(\text{Conv}(I^{\prime}))) \in \bbR^{n \times m \times d_{\text{out}}},
% $$
\begin{align}
    F = \text{Conv}(\text{ReLU}(\text{Conv}(I^{\prime}))) \in \bbR^{n \times m \times d_{\text{out}}},
\end{align}

\subsection{Output Layer}

In the final interaction layer, the global feature maps $F=[F^x, F^{p'}] \in \calR^{n \times m \times 2}$ are obtained and used to compute allocation and price through the output layer. Noticing that price $\bmp \in \calR^{m}$, we need to cut down buyer dimension of  feature map $F^{p'}$ by just take an average on all the buyers. 
% $$F^p_j = \frac{1}{n}F^{p'}_{\cdot,j}$$
\begin{align}
    F^p_j = \frac{1}{n}F^{p'}_{\cdot,j}
\end{align}
Once the output shape matches,  we can make the final allocation and price by doing some simple Softmax, which is briefly introduced in the main body.  

The Softmax function 
% $$\text{softmax}(x)_i = \frac{e^{x_i}}{\sum_{j=1}^n e^{x_j}}
% $$
\begin{align}
    \text{softmax}(x)_i = \frac{e^{x_i}}{\sum_{j=1}^n e^{x_j}}
\end{align}
has some wonderful properties. firstly, it normalizes all the input values and then makes sure they sum to $1$.  Secondly, The exponential form of the function inside Softmax ensures that its output is greater than 0. In addition, It guarantees that it is derivable, which is useful for back-propagation. 

By taking Softmax operation on goods shown as below,
\begin{align}
    \bmx_{\cdot,j} &= \text{Softmax}(F^x_{\cdot,j}) \times n, \quad \forall j \in [m]. \\
\end{align}
One can confidently say that the sum of allocation $\bmx_{\cdot,j} = 1*n$, which means that the total allocation of good $j$ is equal to its initial endowment n, which is the number of buyers. And we give everyone a non-negative number of good j, In terms of the formula is $\bmx_{ij} \ge 0$.

Same thing happens to price:
% $$\bmp_{\cdot} = \text{Softmax}(F^p_{\cdot}) \times \frac{1}{n}\sum_{i=1}^n B(b_i).$$
\begin{align}
    \bmp_{\cdot} = \text{Softmax}(F^p_{\cdot}) \times \frac{1}{n}\sum_{i=1}^n B(b_i).
\end{align}
By this transformation, we can reach the constraint $n \sum_{j=1}^m \bmp = \sum_{i=1}^n B(b_i)$, which means that the value of all items equals the sum of all buyers' budgets (recall we have n pieces of good $j, \ \forall j \in [m]$). 

\subsection{Some Issues on Optimization}

To compute $\GAP(\bmx,\bmp)$, it is required to access the Fixed-price utility $\tilde{u}(b_i;\bmp)$.
We derive the explicit expressions of $u(b_i;\bmp)$ for CES utility functions in \cref{app:derivation}. 
For those utility functions that do not equip with an explicit formula, we argue that it's still possible that
% we have an approximation of $\GAP(\bmx,\bmp)$, and 
MarketTransNet works. 
% The details are moved to \cref{app:trans-architecture} and we do not consider this case in our experiments.

% \section{The case \texorpdfstring{$\Tilde{u}(b;\bmp)$}{} does not obtain a closed form}

The theme point is to obtain a measure for market equilibrium without directly computing fixed-price utility. The term $B_i (\log \Tilde{u}_i(\bmp) - \log u_i(\bmx_i))$ in GAP draws the buyer optimality disobey if $\langle \bmp, \bmx_i\rangle = B_i$. 
However, it does not generally hold that $\langle \bmp, \bmx_i\rangle = B_i$ even if market clearance and price constraints hold.

In the proof of \cref{prf:thm:gap-largerthan0}, we denote $B'_i = \langle \bmp, \bmx_i\rangle$ and $\bmx'_i = \frac{B_i}{B'_i} \bmx_i$. If we ignore the KL divergence term, then the GAP is directly
\begin{align}
    \sum_\iinn B_i(\log \Tilde{u}_i(\bmp) - \log u_i(\bmx'_i))
\end{align}

where $\log \Tilde{u}_i(\bmp) - \log u_i(\bmx'_i)$ can be seen as the regret for buyer $i$. Even though the regret may not have a closed form (since we assume that $\Tilde{u}(b;\bmp)$ does not obtain a closed form), we may achieve a closed form of the gradient of the regret (or calculated by autograd module in pytoch), i.e.

\begin{align}
    \nabla \log u_i(\bmx'_i) =& \lim_{\bmx''_i \to \bmx'_i} \frac{\log u_i(\bmx''_i) - \log u_i(\bmx'_i)}{||\bmx''_i - \bmx'_i||}
    \\
    \st& \quad \bmx''_i \ge 0,\quad \langle \bmx''_i ,\bmp\rangle = B_i
\end{align}

Therefore, we can also minimize 
\begin{align}
    \GAP' = \sum_\iinn B_i ||\nabla \log u_i(\bmx'_i)||^2
\end{align}

and $\GAP' = 0$ if and only if $(\bmx'_i, \bmp)$ constitutes a market equilibrium. To make sure $\bmx'_i = \bmx_i$ for all $i$, we can add the KL divergence term back to penalize the difference between $\bmx$ and $\bmx'_i$.
