# Supplementary material for: Large-Scale Contextual Market Equilibrium Computation through Deep Learning
Source: arXiv:2406.15459 source file (2025-04-21)
Supplement: Supplementary file 3 [file Utility.tex]

% \section{CCNH Utility Functions}

% \myx{Revise}In this paper, we mainly consider four kinds of CCNH utility functions that are widely acknowledged in the mainstream of economics literature \citep[\S 6.1.5]{nisan2007algorithmic}.
% \begin{itemize}
%     \item linear utility, \ie, $u(b_i;\bmx_i) = \sum_\jinm v(b_i, g_j) x_{ij}$,
%     where $v(b_i,g_j)$ (same below) can be explained as the value of item $j$ $i$ to buyer.

%     \item Leontief utility, $u(b_i; \bmx_i) = \min_\jinm v(b_i,g_j) x_{ij}$.

%     \item Cobb-Douglas utility, $u(b_i;\bmx_i) = \prod_\jinm x_{ij}^{v(b_i,g_j)}$, where $\sum_\jinm v(b_i,g_j) = 1$.

%     \item general Constant Elasticity of Substitution(CES) utility with degree $\alpha \le 1$\citep{CES:varian1992microeconomic},
%     \begin{align}
%         u(b_i;\bmx_i) = \left( \sum_\jinm v^\alpha(b_i,g_j) x_{ij}^\alpha \right)^{1/\alpha}
%     \end{align}
%     % where $v_{\mathrm{total}}(b_i) = 1 / \sum_\jinm v'(b_i,g_j)$.
% \end{itemize}

% For CES functions, \citet{CES-general:arrow1961capital} has shown that, linear, Cobb-Douglas as well as Leontief utility functions are special cases of CES functions in the limit, which states as the next proposition.

% \begin{proposition}
% \label{pro:CES-is-enough}
% We have following statements.
% \begin{itemize}
%     \item Linear utility can be represented by a CES utility with $\alpha=1$

%     \item Leontief utility can be represented by a CES utility with $\alpha \to -\infty$.

%     \item Cobb-Douglas utility can be represented by a CES utility with $\alpha \to 0$.

%     \item CES utility satisfies CCNH condition when $\alpha \le 1$.
% \end{itemize}
% \end{proposition}

% For completeness of the paper, we present a self-contained proof in \cref{app:proofs}.

% Inspired by \cref{pro:CES-is-enough}, we focus on CES utility function with $\alpha \le 1$ from now on. 
